# Supplementary material for: Interaction-aware Model Predictive Control for Autonomous Driving
Source: arXiv:2211.17053 source file (2022-11-30)
Supplement: Supplementary file 1 [file Appendix.tex]

\subsection{Influence of Initialization}
A good initialization of $\param_0$ will greatly influence the performance.
